# Supplementary material for: Safe Explicable Policy Search
Source: arXiv:2503.07848 source file (2025-09-25)
Supplement: Supplementary file 1 [file appendix.pdf]

# Analytical solution for SEPS

The SEPS problem is approximated by

$$\begin{aligned}
 \theta_{n+1} &= \arg \max_{\theta} g^T(\theta - \theta_n) \\
 \text{s.t. } &c_0 - b_0^T(\theta - \theta_n) \leq 0 \\
 &c_i + b_i^T(\theta - \theta_n) \leq 0 \quad i = 1, \dots, k \\
 &\frac{1}{2}(\theta - \theta_n)^T H(\theta - \theta_n) \leq \delta
 \end{aligned} \tag{1}$$

Let  $x = \theta - \theta_n$ . Here, we derive the solution for the special case with a single cost function  $C_1$  which results in a total of two constraints. The resulting objective with linear and quadratic constraints is discussed under the feasible and infeasible case.

## 0.1 Feasible case

**Theorem 1** *Consider the following problem*

$$\begin{aligned}
 p^* &= \min_x g^T x \\
 \text{s.t. } &b_0^T x + c_0 \leq 0 \\
 &b_1^T x + c_1 \leq 0 \\
 &\frac{1}{2}x^T H x \leq \delta
 \end{aligned}$$

where  $g, b, x \in \mathbb{R}^l, c, \delta \in \mathbb{S}^l$  and  $H \succ 0$ . When there is at least one strictly feasible point, the optimal point  $x^*$  satisfies the following condition

$$x^* = -\frac{1}{\lambda^*} H^{-1} (g + \nu_0^* b_0 + \nu_1^* b_1)$$

where,  $\lambda^*, \nu_0^*$ , and  $\nu_1^*$  are defined by

case 1: When  $\nu_0 > 0$  and  $\nu_1 > 0$

$$\nu_0^* = \frac{\lambda c_0 - \nu_1 t - r_0}{s_0} \quad \nu_1^* = \frac{\lambda c_1 - \nu_0 t - r_1}{s_1}$$

$$\lambda^* = \arg \max_{\lambda \geq 0} \begin{cases} f_1(\lambda) & \text{if } \frac{\lambda(s_1 c_0 - t c_1) + t r_1 - s_1 r_0}{s_0 s_1 - t^2} > 0 \text{ and } \frac{\lambda(s_0 c_1 - t c_0) + t r_0 - s_0 r_1}{s_0 s_1 - t^2} > 0 \\ f_4(\lambda) & \text{otherwise} \end{cases}$$

case 2: When  $\nu_0 > 0$  and  $\nu_1 = 0$

$$\begin{aligned}\nu_0^* &= \frac{\lambda c_0 - r_0}{s_0} & \nu_1^* &= 0 \\ \lambda^* &= \arg \max_{\lambda \geq 0} \begin{cases} f_2(\lambda) & \text{if } \frac{\lambda c_0 - r_0}{s_0} > 0 \\ f_4(\lambda) & \text{otherwise} \end{cases}\end{aligned}$$

Case 3: When  $\nu_0 = 0$  and  $\nu_1 > 0$

$$\begin{aligned}\nu_0^* &= 0 & \nu_1^* &= \frac{\lambda c_1 - r_1}{s_1} \\ \lambda^* &= \arg \max_{\lambda \geq 0} \begin{cases} f_3(\lambda) & \text{if } \frac{\lambda c_1 - r_1}{s_1} > 0 \\ f_4(\lambda) & \text{otherwise} \end{cases}\end{aligned}$$

Case 4: When  $\nu_0 = 0$  and  $\nu_1 = 0$

$$\begin{aligned}\nu_0^* &= 0 & \nu_1^* &= 0 \\ \lambda^* &= \max_{\lambda \geq 0} f_4(\lambda)\end{aligned}$$

where,

$$\begin{aligned}f_1(\lambda) &\doteq \frac{1}{2\lambda}(-q) + \frac{\lambda}{2} \left( \frac{s_1 c_0^2 + s_0 c_1^2 - 2t c_0 c_1}{s_0 s_1 - t^2} - 2\delta \right) \\ &+ \frac{tr_1 c_0 + tr_0 c_1 - s_1 r_0 c_0 - s_0 r_1 c_1 - s_1 r_0^2 - s_0 r_1^2 + 2tr_0 r_1}{s_0 s_1 - t^2} \\ f_2(\lambda) &\doteq \frac{1}{2\lambda} \left( \frac{r_0^2}{s_0} - q \right) + \frac{\lambda}{2} \left( \frac{c_0^2}{s_0} - 2\delta \right) - \frac{r_0 c_0}{s_0} \\ f_3(\lambda) &\doteq \frac{1}{2\lambda} \left( \frac{r_1^2}{s_1} - q \right) + \frac{\lambda}{2} \left( \frac{c_1^2}{s_1} - 2\delta \right) - \frac{r_1 c_1}{s_1} \\ f_4(\lambda) &\doteq \frac{1}{2\lambda}(-q) + \frac{\lambda}{2}(-2\delta)\end{aligned}$$

with  $q = g^T H^{-1} g$ ,  $r_0 = g^T H^{-1} b_0$ ,  $r_1 = g^T H^{-1} b_1$ ,  $s_0 = b_0^T H^{-1} b_0$ ,  $s_1 = b_1^T H^{-1} b_1$ ,  $t = b_0^T H^{-1} b_1$ .

**Proof:** This is a convex optimization problem. When there is at least one strictly feasible point, strong duality holds by Slater's theorem. The dual to the above problem is

$$p^* = \min_x \max_{\lambda \geq 0, \nu_0 \geq 0, \nu_1 \geq 0} g^T x + \lambda \left( \frac{1}{2} x^T H x - \delta \right) + \nu_0 (b_0^T x + c_0) + \nu_1 (b_1^T x + c_1) \quad (2)$$

$$= \max_{\lambda \geq 0, \nu_0 \geq 0, \nu_1 \geq 0} \min_x \frac{\lambda}{2} x^T H x + (g^T + \nu_0 b_0^T + \nu_1 b_1^T) x + \nu_0 c_0 + \nu_1 c_1 - \lambda \delta \quad (3)$$

(Strong duality)

$$\frac{\partial \mathcal{L}(x, \lambda, \nu_0, \nu_1)}{\partial x} = \frac{\lambda}{2} 2xH + g + \nu_0 b_0 + \nu_1 b_1$$

(Stationarity condition)  $\{\frac{\partial L}{\partial x} = 0\}$

$$\therefore x^* = -\frac{1}{\lambda} H^{-1} (g + \nu_0 b_0 + \nu_1 b_1)$$

Substitute  $x^*$  in Eq. (3):

$$\begin{aligned} p^* &= \max_{\lambda \geq 0, \nu_0 \geq 0, \nu_1 \geq 0} \frac{\lambda}{2} \left( \frac{-1}{\lambda} H^{-1} (g + \nu_0 b_0 + \nu_1 b_1) \right)^T H \left( \frac{-1}{\lambda} H^{-1} (g + \nu_0 b_0 + \nu_1 b_1) \right) \\ &\quad + (g^T + \nu_0 b_0^T + \nu_1 b_1^T)^T \left( \frac{-1}{\lambda} H^{-1} (g + \nu_0 b_0 + \nu_1 b_1) \right) + \nu_0 c_0 + \nu_1 c_1 - \lambda \delta \\ &= \max_{\lambda \geq 0, \nu_0 \geq 0, \nu_1 \geq 0} -\frac{1}{2\lambda} (g^T H^{-1} g + \nu_0 g^T H^{-1} b_0 + \nu_1 g^T H^{-1} b_1 + \nu_0 b_0^T H^{-1} g + \nu_0^2 b_0^T H^{-1} b_0 \\ &\quad + \nu_0 \nu_1 b_0^T H^{-1} b_1 + \nu_0 \nu_1 b_0^T H^{-1} b_1 + \nu_1 b_1^T H^{-1} g + \nu_0 \nu_1 b_1^T H^{-1} b_0 + \nu_1^2 b_1^T H^{-1} b_1) \\ &\quad + \nu_0 c_0 + \nu_1 c_1 - \lambda \delta \\ &\quad \text{Let } q = g^T H^{-1} g, r_0 = g^T H^{-1} b_0, r_1 = g^T H^{-1} b_1, s_0 = b_0^T H^{-1} b_0, \\ &\quad s_1 = b_1^T H^{-1} b_1, t = b_0^T H^{-1} b_1 \\ &= \max_{\lambda \geq 0, \nu_0 \geq 0, \nu_1 \geq 0} -\frac{1}{2\lambda} (q + 2\nu_0 r_0 + 2\nu_1 r_1 + \nu_0^2 s_0 + \nu_1^2 s_1 + 2\nu_0 \nu_1 t) \\ &\quad + \nu_0 c_0 + \nu_1 c_1 - \lambda \delta \quad (4) \end{aligned}$$

Case 1: When  $\nu_0 > 0$  and  $\nu_1 > 0$

Here, both constraints are active.

Optimizing single-variable convex quadratic function over  $\mathbb{R}_+$  for  $\nu_0$   
(i.e. for fixed value of  $\lambda$  and  $\nu_1$  find the value of  $\nu_0$ )

$$\frac{\partial \mathcal{L}(\lambda, \nu_0, \nu_1)}{\partial \nu_0} = -\frac{1}{2\lambda} (2r_0 + 2\nu_0 s_0 + 2\nu_1 t) + c_0$$

$$\frac{\partial L}{\partial \nu_0} = 0$$

$$\therefore \nu_0 = \frac{\lambda c_0 - \nu_1 t - r_0}{s_0} \quad (5)$$

Optimizing single-variable convex quadratic function over  $\mathbb{R}_+$  for  $\nu_1$

(i.e. for fixed value of  $\lambda$  and  $\nu_0$  find the value of  $\nu_1$ )

$$\frac{\partial \mathcal{L}(\lambda, \nu_0, \nu_1)}{\partial \nu_1} = -\frac{1}{2\lambda} (2r_1 + 2\nu_1 s_1 + 2\nu_0 t) + c_1$$

$$\frac{\partial L}{\partial \nu_1} = 0$$

$$\therefore \nu_1 = \frac{\lambda c_1 - \nu_0 t - r_1}{s_1} \quad (6)$$

Solving Eq. 5 and Eq. 6 simultaneously, we get

$$\therefore \nu_0 = \frac{\lambda(s_1 c_0 - t c_1) + t r_1 - s_1 r_0}{s_0 s_1 - t^2} \quad (7)$$

$$\therefore \nu_1 = \frac{\lambda(s_0 c_1 - t c_0) + t r_0 - s_0 r_1}{s_0 s_1 - t^2} \quad (8)$$

Substitute the values of  $\nu_0$  and  $\nu_1$  above in Eq. (4), we get

$$p^* = \max_{\lambda \geq 0} f_1(\lambda) = \frac{1}{2\lambda} (-q) + \frac{\lambda}{2} \left( \frac{s_1 c_0^2 + s_0 c_1^2 - 2t c_0 c_1}{s_0 s_1 - t^2} - 2\delta \right) + \frac{t r_1 c_0 + t r_0 c_1 - s_1 r_0 c_0 - s_0 r_1 c_1 - s_1 r_0^2 - s_0 r_1^2 + 2t r_0 r_1}{s_0 s_1 - t^2} \quad (9)$$

Optimize Eq. (9) if  $\lambda \in \Lambda_1$ , where

$$\Lambda_1 = \left\{ \lambda \left| \frac{\lambda(s_1 c_0 - t c_1) + t r_1 - s_1 r_0}{s_0 s_1 - t^2} > 0, \frac{\lambda(s_0 c_1 - t c_0) + t r_0 - s_0 r_1}{s_0 s_1 - t^2} > 0, \lambda \geq 0 \right. \right\}$$

Case 2: When  $\nu_0 > 0$  and  $\nu_1 = 0$

Here, the 1<sup>st</sup> constraint is active and the 2<sup>nd</sup> constraint is inactive.

Set  $\nu_1 = 0$  in Eq. (4), we get

$$p^* = \max_{\lambda \geq 0, \nu_0 \geq 0} -\frac{1}{2\lambda} (q + 2\nu_0 r_0 + \nu_0^2 s_0) + \nu_0 c_0 - \lambda \delta \quad (10)$$

$$\frac{\partial L}{\partial \nu_0} = 0$$

$$\therefore \nu_0 = \frac{\lambda c_0 - r_0}{s_0} \quad (11)$$

Substitute the value of  $\nu_0$  above in Eq. 10, we get

$$p^* = \max_{\lambda \geq 0} f_2(\lambda) = \frac{1}{2\lambda} \left( \frac{r_0^2}{s_0} - q \right) + \frac{\lambda}{2} \left( \frac{c_0^2}{s_0} - 2\delta \right) - \frac{r_0 c_0}{s_0} \quad (12)$$

Optimize Eq. (12) if  $\lambda \in \Lambda_2$ , where

$$\Lambda_2 = \left\{ \lambda \left| \frac{\lambda c_0 - r_0}{s_0} > 0, \lambda \geq 0 \right. \right\}$$

Case 3: When  $\nu_0 = 0$  and  $\nu_1 > 0$

Here, the 1<sup>st</sup> constraint is inactive and the 2<sup>nd</sup> constraint is active. Set  $\nu_0 = 0$  in Eq. (4), we get

$$p^* = \max_{\lambda \geq 0, \nu_1 \geq 0} -\frac{1}{2\lambda} (q + 2\nu_1 r_1 + \nu_1^2 s_1) + \nu_1 c_1 - \lambda \delta \quad (13)$$

$$\frac{\partial L}{\partial \nu_1} = 0$$

$$\therefore \nu_1 = \frac{\lambda c_1 - r_1}{s_1} \quad (14)$$

Substitute the value of  $\nu_1$  above in Eq. 13, we get

$$p^* = \max_{\lambda \geq 0} f_3(\lambda) = \frac{1}{2\lambda} \left( \frac{r_1^2}{s_1} - q \right) + \frac{\lambda}{2} \left( \frac{c_1^2}{s_1} - 2\delta \right) - \frac{r_1 c_1}{s_1} \quad (15)$$

Optimize Eq. (15) if  $\lambda \in \Lambda_3$ , where

$$\Lambda_3 = \left\{ \lambda \left| \frac{\lambda c_1 - r_1}{s_1} > 0, \lambda \geq 0 \right. \right\}$$

Case 4: When  $\nu_0 = 0$  and  $\nu_1 = 0$

Here, both constraints are inactive.

Set  $\nu_0 = 0$  and  $\nu_1 = 0$  in Eq. (4), we get

$$p^* = \max_{\lambda \geq 0} f_4(\lambda) = \frac{1}{2\lambda} (-q) + \frac{\lambda}{2} (-2\delta) \quad (16)$$

Optimize Eq. (16) if  $\lambda \in \Lambda_4$ , where

$$\Lambda_4 = \left\{ \lambda \left| \frac{\lambda(s_1 c_0 - t c_1) + t r_1 - s_1 r_0}{s_0 s_1 - t^2} \leq 0, \frac{\lambda(s_0 c_1 - t c_0) + t r_0 - s_0 r_1}{s_0 s_1 - t^2} \leq 0, \right. \right. \\ \left. \left. \frac{\lambda c_0 - r_0}{s_0} \leq 0, \frac{\lambda c_1 - r_1}{s_1} \leq 0, \lambda \geq 0 \right\}$$

In summary, solving the dual for  $\lambda$ : for any  $A > 0$ ,  $B > 0$ , the problem

$$\max_{\lambda \geq 0} f(\lambda) = -\frac{1}{2} \left( \frac{A}{\lambda} + B\lambda \right) \quad (17)$$

has optimal point  $\lambda^* = \sqrt{A/B}$  and optimal value  $f(\lambda^*) = \sqrt{AB}$ .

If  $\lambda^*$ ,  $\nu_0^*$ , and  $\nu_1^*$  are a solution to the dual above. The update rule for the feasible case is

$$\theta_{n+1} = \theta_n - \frac{1}{\lambda} H^{-1} (g + \nu_0 b_0 + \nu_1 b_1) \quad (18)$$

## 0.2 Infeasible case

**Theorem 2** Consider the following problem

$$\begin{aligned} \hat{p} = \min_{\theta} \quad & c_m - b_m^T(\theta - \theta_n) \\ \text{s.t.} \quad & \frac{1}{2}(\theta - \theta_n)^T H(\theta - \theta_n) \leq \delta \end{aligned}$$

where  $m \in [0, k]$ ,  $b, x \in \mathbb{R}^l$ ,  $c, \delta \in \mathbb{S}^l$  and  $H \succ 0$ . When there is at least one strictly feasible point, the optimal point  $x^*$  satisfies the following condition

$$x^* = -\frac{1}{\phi^*} H^{-1} b_m$$

where,  $\phi^*$  is defined by

$$\phi^* = \sqrt{\frac{s}{2\delta}}$$

with  $s = b_m^T H^{-1} b_m$ .

**Proof:** This is a convex optimization problem. When there is at least one strictly feasible point, strong duality holds by Slater's theorem. The dual to the above problem is

$$\hat{p} = \min_x \max_{\phi \geq 0} b_m^T x + c_m + \phi \left( \frac{1}{2} x^T H x - \delta \right) \quad (19)$$

$$\hat{p} = \max_{\phi \geq 0} \min_x \frac{\phi}{2} x^T H x + b_m^T x + c_m - \phi \delta \quad (20)$$

(Strong duality)

$$\frac{\partial \mathcal{L}(x, \phi)}{\partial x} = \frac{\phi}{2} 2xH + b_m$$

(Stationarity condition)  $\left\{ \frac{\partial \mathcal{L}}{\partial x} = 0 \right\}$

$$\therefore x^* = -\frac{1}{\phi} H^{-1} b_m$$

Substitute  $x^*$  in Eq. 20:

$$\begin{aligned} \hat{p} &= \max_{\phi \geq 0} \frac{\phi}{2} \left( \frac{-1}{\phi} H^{-1} b_m \right)^T H \left( \frac{-1}{\phi} H^{-1} b_m \right) + b_m^T \left( \frac{-1}{\phi} H^{-1} b_m \right) + c_m - \phi \delta \\ &= \max_{\phi \geq 0} -\frac{b_m^T H^{-1} b_m}{2\phi} + c_m - \phi \delta \end{aligned}$$

Let  $s = b_m^T H^{-1} b_m$ .

$$= \max_{\phi \geq 0} -\frac{s}{2\phi} + c_m - \phi \delta$$

$$\frac{\partial \mathcal{L}(\phi)}{\partial \phi} = -\frac{s}{2} \left( -\frac{1}{\phi^2} \right) - \delta$$

$$\text{(Stationarity condition) } \left\{ \frac{\partial \mathcal{L}}{\partial \phi} = 0 \right\}$$

$$\therefore \phi^* = \sqrt{\frac{s}{2\delta}}$$

If  $\phi^*$  is the solution to the dual above. The update rule for the infeasible case is

$$\theta_{n+1} = \theta_n - \sqrt{\frac{2\delta}{s}} H^{-1} b_m \quad (21)$$
